# Supplementary material for: Intermittent Visual Servoing: Efficiently Learning Policies Robust to Instrument Changes for High-precision Surgical Manipulation
Source: arXiv:2011.06163 source file (2020-11-12)
Supplement: Supplementary file 1 [file 8_appendix.tex]

\normalsize
We structure this appendix as follows:

\daniel{Insert details here ... maybe details on the robot arms used or hyperparameters used for neural network ensemble.}

\begin{figure}[t]
\centering
\includegraphics[width=1.0\linewidth]{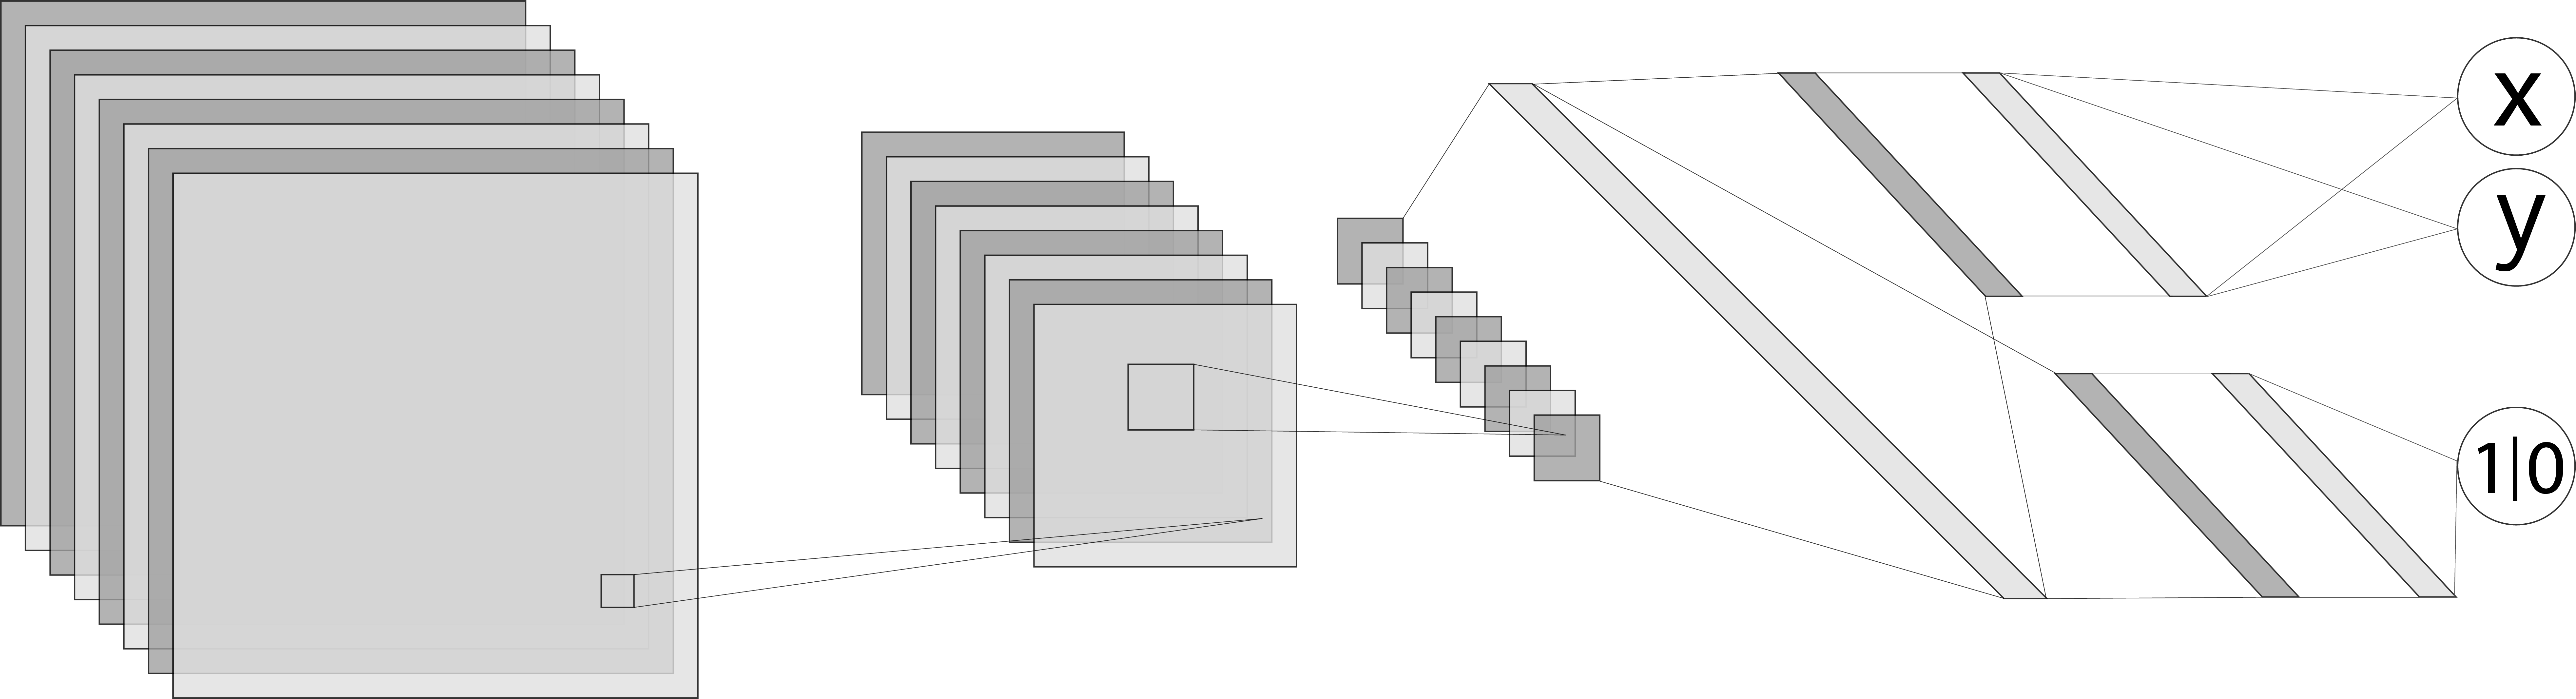}
\caption{
\textbf{Model Visulization.} Each model consists of alternating convolutions and max pools, following by dense layers separated by Dropout and ReLUs. Each model uses a processed 150$\times$150 image $I_t$ as input, and regresses the corrective direction $a_t$ and classifies the completion status $\phi_t$. The weights in the convolutional layers are shared, while the dense layers are independently learned. Sharing convolutional layers helps with performance, as the convolutional filters get two sources of supervision during training. 
% \daniel{TODO: show ensemble a bit more clearly? The input image should also be what we actually pass as input, right now this is too much like MNIST style networks.}
} 
\label{fig:model}
\end{figure}
